# Supplementary material for: Dilatancy-induced fluid pressure drop during dynamic rupture: Direct experimental evidence and consequences for earthquake dynamics
Source: arXiv:1904.10906 ancillary file (2020-03-10)
Supplement: Supplementary file 1 [file sm.pdf]

# Dilatancy-induced fluid pressure drop during dynamic rupture: Direct experimental evidence and consequences for earthquake dynamics [Supplementary materials]

Nicolas Brantut
Department of Earth Sciences
University College London
London, WC1E6BS, UK

## Triaxial apparatus

The jacketed sample was placed inside the pressure vessel of the triaxial apparatus. The confining medium is silicon oil, and the confining pressure is raised by an electro-mechanical pump, and measured with a pressure transducer with a precision of 0.01 MPa. The interstitial pore fluid (here, distilled water) is servo-controlled with a servo-hydraulic intensifier with a precision of 0.01 MPa. The pore fluid intensifier can be connected to either both ends of the sample, or only the top (upstream), leaving the bottom end (downstream) isolated, in contact with a small volume reservoir of calibrated effective compressibility equal to $6 \times 10^{-15}$ m$^3$Pa$^{-1}$. The upstream and downstream fluid pressure, denoted respectively $P_{\mathrm{f,up}}$ and $P_{\mathrm{f,down}}$, are measured by two independent pressure transducers. The axial load is applied by a vertical self-compensated piston, actuated by a servo-controlled hydraulic ram (maximum capacity 1500 kN). The load is measured with an external load cell, and corrected for internal seal friction. Axial shortening is measured by averaging the readings of two external linear variable differential transducers; sample shortening is computed by correcting the external measurements from the elastic strain in the loading column (stiffness 480 kN mm$^{-1}$). The deformation tests were performed under constant a axial deformation rate of $10^{-6}$ s$^{-1}$.

## Detailed geometry and results of sample tested at $P_{\mathrm{c}} = 60$ MPa and $P_{\mathrm{f}} = 20$ MPa

The sample tested at $P_{\mathrm{c}} = 60$ MPa and $P_{\mathrm{f}} = 20$ MPa was initially prepared in the exact same way as the one tested at $P_{\mathrm{c}} = 70$ MPa and $P_{\mathrm{f}} = 30$ MPa (cored, ground, notched and thermally cracked at 600°C). The sample was then equipped with four pore pressure transducers, arranged as shown in Figure S1.

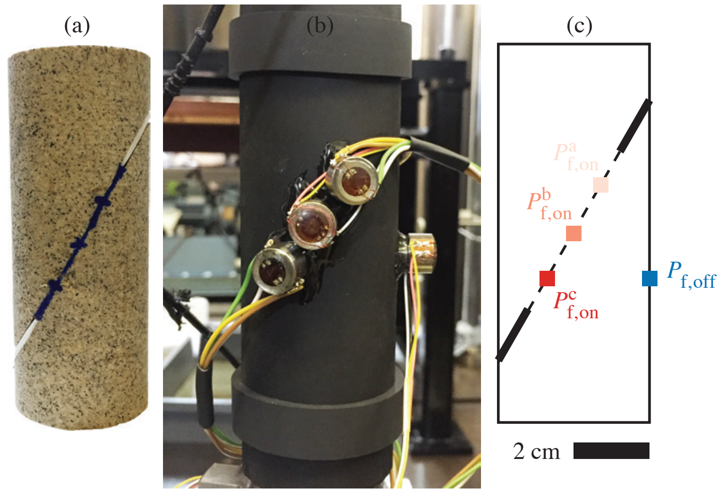


Figure S1: Geometry of sample tested at $P_c$ = 60 MPa and $P_f$ = 20 MPa. (a) Photograph of intact specimen after notch preparation and thermal cracking. (b) Photograph of jacketed sample with pore pressure transducers. (c) Schematic showing sensor positions projected onto the sample's crosss-section.

# Fluid pressure measurements

The fluid pressure transducers were calibrated in situ by changing the uniform pore pressure in the sample while keeping the confining pressure constant (Figure S3). A very satisfactory linear output is observed for all transducers. Two sets of transducers were used, one for which the output was −852 and −827 mV/V per megapascal fluid pressure (shown in Figure S3, used in the test conducted at 70 MPa confining pressure and 30 MPa pore pressure), and others for which the output was −678 and −705 mV/V per megapascal fluid pressure (used only in the test conducted at 60 MPa confining pressure and 20 MPa pore pressure, at positions labelled $P^{a}_{f,on}$ and $P^{c}_{f,on}$ in Figure S1c).

# Wave velocity measurements

The piezoeletric transducers were connected to a 40 dB high-pass preamplifiers, and to 50 MHz digital oscilloscopes. Repeatedly during the experiment, a 250 V, 1 MHz pulse was sent sequentially to each piezoelectric transducer and the resulting signals were recorded on the remaining transducers. The time-of-flight between each pair of transducers was picked manually on a set of reference waveforms obtained during one such survey, and relative variations in time-of-flight were computed automatically by cross-correlation of subsequent waveforms with the reference ones. The wave speed was computed by dividing the distance between each pair of transducers by the corresponding time-of-flight. In terms of wave speed, the absolute accuracy of this method is limited by the quality of the manual picks of the reference waveforms, and is of around 150 m $s^{-1}$. The relative accuracy between successive measurements obtained from cross-correlations is limited by noise in the data and is of around 0.4%.

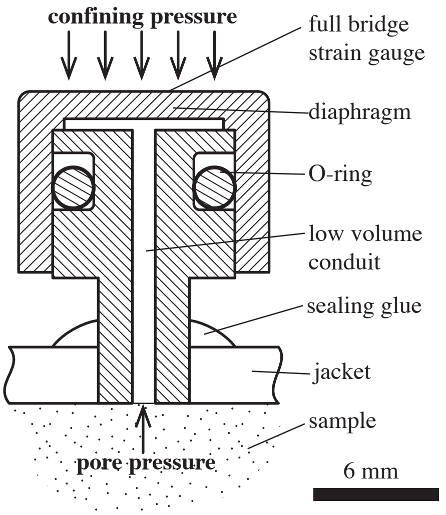


Figure S2: Schematic cross-section of the fluid pressure (differential) transducers. The circular surface of the steel cap is bonded to a full bridge diaphragm strain gauge that measures the elastic distortion of the cap due to the pressure difference between the confining medium (directly in contact with the cap surface) and the pore fluid pressure (connected to the sample's pore space through a small internal conduit).

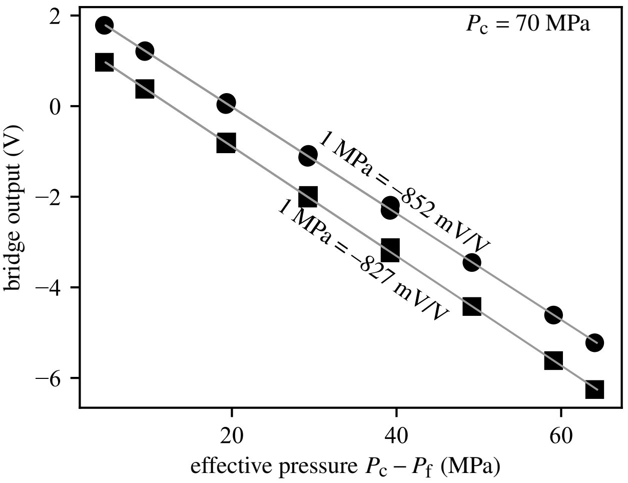


Figure S3: Bridge output of the fluid pressure transducers as a function of pore pressure (after homogeneisation of fluid pressure within the sample), under a constant confining pressure $P_c = 70$ MPa.

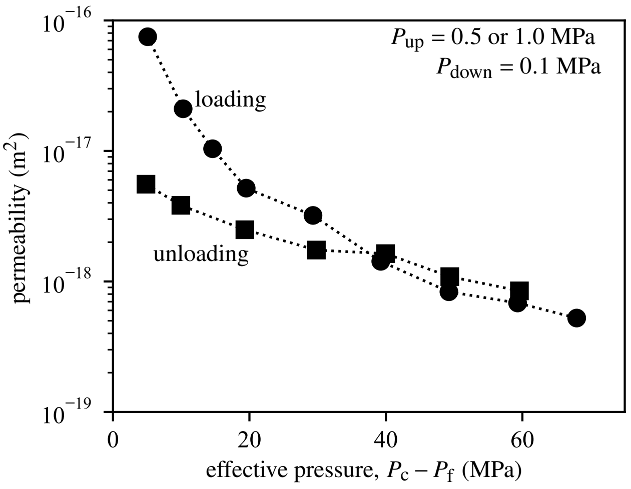


Figure S4: Permeability during hydrostatic pressurisation/depressurisation cycle, measured using the constant flow rate method.

# Sample characterisation

Prior to deformation and fracture, the poro-elastic and hydraulic properties of the sample were characterised during a series of hydrostatic loading and unloading cycles.

A first hydrostatic pressurisation cycle was conducted from $P_{\mathrm{c}} = 5$ to 70 MPa, while imposing an upstream pore pressure $P_{\mathrm{f,up}} = 0.5$ MPa and venting the downstream pore pressure outlet ($P_{\mathrm{f,down}} = 0.0$ MPa). The permeability of the sample was computed from the measurements of steady-state flow rate during each pressure step. The starting permeability at $P_{\mathrm{c}} = 5$ MPa is of $7 \times 10^{-17}$ m$^2$, and decreases nonlinearly down to $5 \times 10^{-19}$ m$^2$ at $P_{\mathrm{c}} = 70$ MPa (Figure S4). During unloading, the permeability increases to $5 \times 10^{-18}$ m$^2$ when the confining pressures is decreased back to 5 MPa.

The downstream pore pressure outlet was then connected to the pore pressure intensifier, and a uniform pore pressure $P_{\mathrm{f,up}} = P_{\mathrm{f,down}} = 1$ MPa was set. The confining pressure was increased stepwise up to $P_{\mathrm{c}} = 70$ MPa, and at each step the bulk volumetric strain $\Delta V_{\mathrm{bulk}}/V_{\mathrm{bulk}}$ (from strain gauge data) and pore volume change $\Delta V_{\mathrm{pore}}/V_{\mathrm{bulk}}$ were recorded (Figure S5a). From these data, the pore compressibility $\phi C_{\mathrm{pc}} = (1/V_{\mathrm{bulk}})\partial V_{\mathrm{pore}}/\partial P_{\mathrm{c}}$ and drained bulk compressibility $C_{\mathrm{bc}} = (1/V_{\mathrm{bulk}})\partial V_{\mathrm{bulk}}/\partial P_{\mathrm{c}}$ were computed (Figure S5b).

At $P_{\mathrm{c}} = 70$ MPa, the downstream pore pressure circuit was isolated from the upstream circuit and intensifier. The upstream pore pressure was increased in steps of 10 MPa in magnitude, and during each step the equilibration of fluid pressure across the sample (using measurements of $P_{\mathrm{f,off}}$, $P_{\mathrm{f,on}}$ and $P_{\mathrm{f,down}}$) was monitored. For a step change in upstream pore pressure and diffusion to a closed downstream reservoir, the transient fluid pressure diffusion profile is given by

$$p(y,t) = \Delta p \left[ 1 - \sum_{k=1}^{\infty} \frac{2(\phi_k^2 + \ell^2) e^{-\phi_k^2 t/\tau} \sin(\phi_k y/L)}{\phi_k(\phi_k^2 + \ell^2 + \ell)} \right], \tag{1}$$

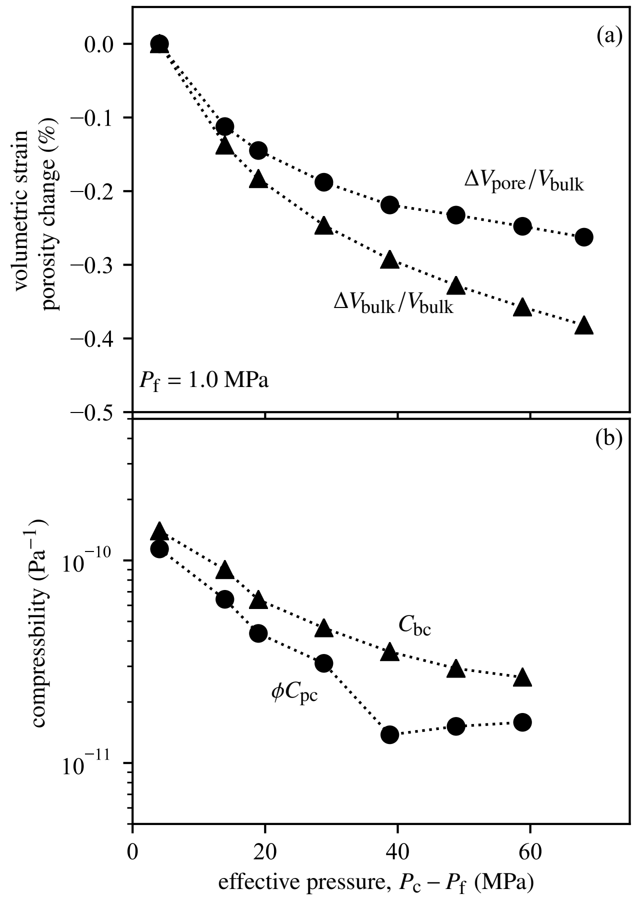


Figure S5: (a) Measurements of pore volume change $\Delta V_{\text{pore}}/V_{\text{bulk}}$ (from pore volumometry) and bulk volume change $\Delta V_{\text{bulk}}/V_{\text{bulk}}$ (from strain gauge measurements) during an increase in confining pressure at constant uniform pore pressure ($P_{\text{f,up}} = P_{\text{f,down}} = 1$ MPa). (b) Drained bulk compressibility and pore compressibility as derived from pore and bulk volume change with increasing confining pressure.

where $y$ is the vertical coordinate along the sample axis ($y = 0$ at the upstream end), $\Delta p$ is the upstream pore pressure change, $\tau = L^2/\alpha_{\mathrm{hy}}$ is the hydraulic diffusion time within the sample, where $L$ is the sample length and $\alpha_{\mathrm{hy}}$ is the hydraulic diffusivity. The quantities $\phi_k$ are the roots of

$$\phi \tan(\phi) = \ell, \tag{2}$$

and the parameter $\ell$ is given by

$$\ell = \beta A L / C_{\mathrm{res}}, \tag{3}$$

where $\beta$ is the storage capacity of the sample, $A$ is its cross sectional area, and $C_{\mathrm{res}}$ is the effective storage capacity of the downstream reservoir. The solution for $p(y, t)$ (Equation 1) can be found from an analogous heat diffusion problem solved in (Carslaw and Jaeger, 1959, chap. 3, p. 129).

The measurements of $P_{\mathrm{f,off}}$, $P_{\mathrm{f,on}}$ and $P_{\mathrm{f,down}}$ provide the time evolution of pore pressure at three different positions $y$ in the sample. The time series are fitted to Equation (1) by a grid-search approach to determine the two quantities $\tau/\ell$ and $\ell$, and obtain an estimate of the sample storage capacity $\beta = \ell C_{\mathrm{res}}/(AL)$ and permeability $k = C_{\mathrm{res}} L \eta/(A\tau/\ell)$. The data and fits are shown in Figure S6, and an independent check is conducted by comparing the measured upstream flow rate and the computed one. The resulting permeability and storage capacity as a function of the (Terzaghi) effective pressure are shown in Figure 1 (right panel) of the main text.

Note that Equation (1) assumes only one dimensional diffusion along the sample axis, and therefore neglects any potential effects of the 30° notches (filled with Teflon). The good match between modelled and observed pore pressure timeseries, in addition to reasonable predictions of fluid volume change (Figure S6) indicates that the potential effects of Teflon-filled notches is negligible here.

The P-wave velocity along different paths was monitored during the hydrostatic pressurisation cycles. Figure S7 shows the horizontal P-wave velocity between the pair of transducers positioned half-way up the sample, as a function of the effective pressure evaluated either at the upstream end ($P_{\mathrm{c}} - P_{\mathrm{f,up}}$, grey curve) or at the middle of the sample ($P_{\mathrm{c}} - P_{\mathrm{f,on}}$, black curve), during the cycle conducted at $P_{\mathrm{c}} = 70$ MPa and step-wise increases in fluid pressure. The P-wave velocity variations along a given ray path are strongly correlated with the *local* fluid pressure (and therefore effective pressure) along that path: as observed in Figure S7, P-wave velocity directly reflects the local fluid pressure but not the upstream (imposed) fluid pressure, which further confirms the validity of the local fluid pressure measurements and justifies the use of specific ray paths as a means to evaluate the local pressure conditions along these paths (e.g., Passelègue et al, 2018).

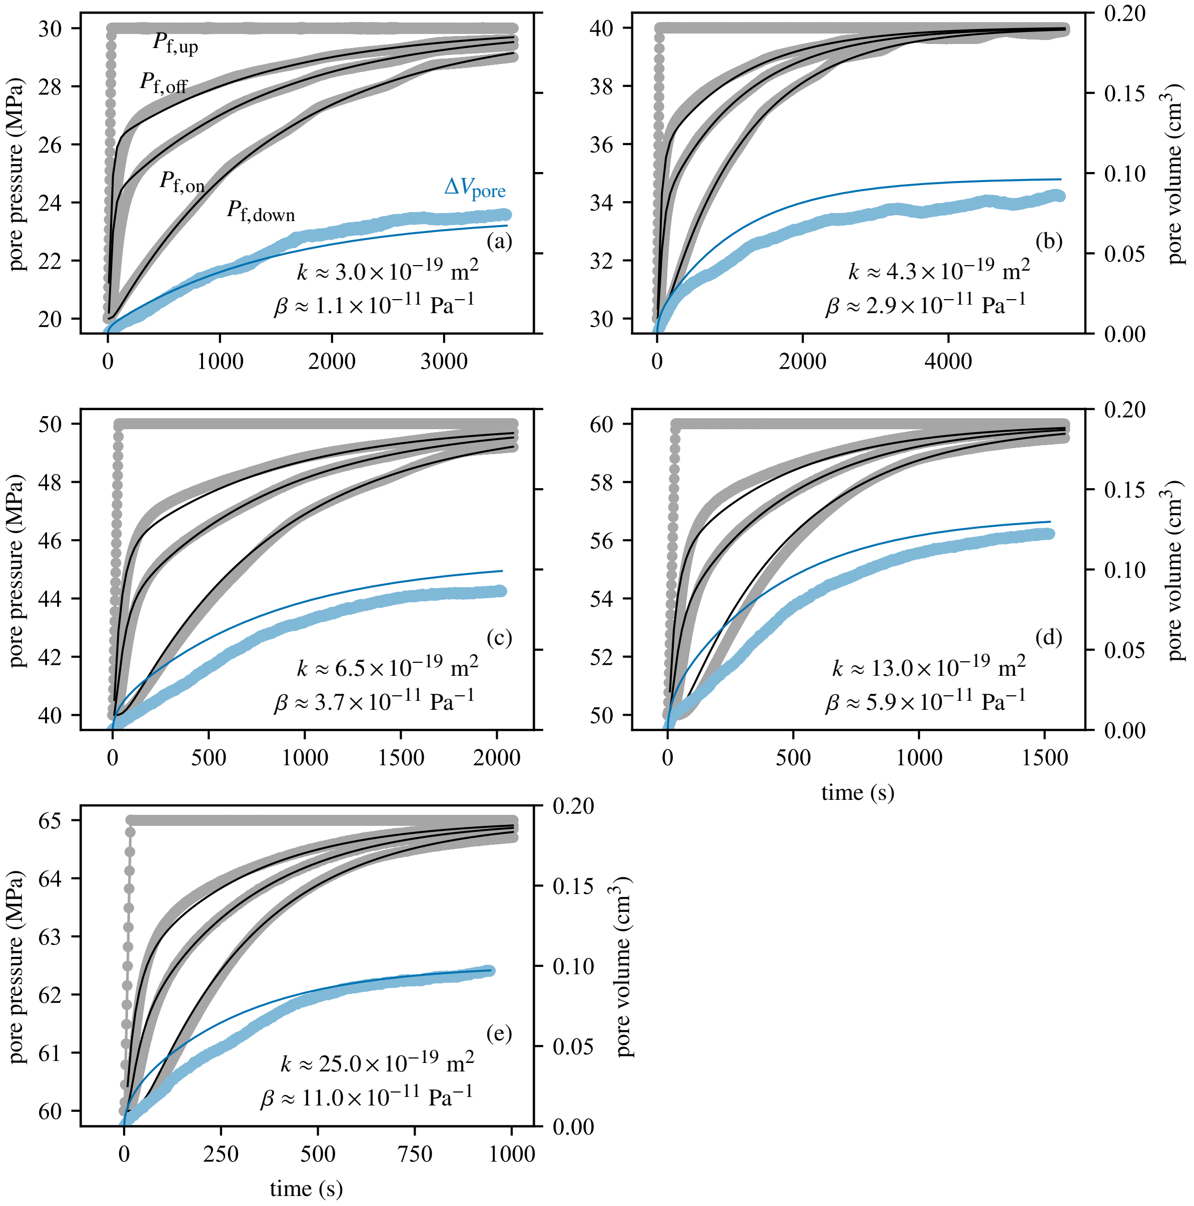


Figure S6: Time series of fluid pressure at different positions along the sample in response to step-wise increases in the upstream fluid pressure, under a constant confining pressure $P_c = 70$ MPa. Panels (a) to (e) correspond each to the pressure and volume records follwing a 10 MPa step from an initial pore pressure of 20 to 60 MPa, respectively. Pressure data are shown in grey, and theoretical values using Equation (1) are shown in black. Pore volume change data are shown in light blue, and the predicted values are shown in thin dark blue lines. The inverted permeability $k$ and storage capacity $\beta$ are displayed in each panel.

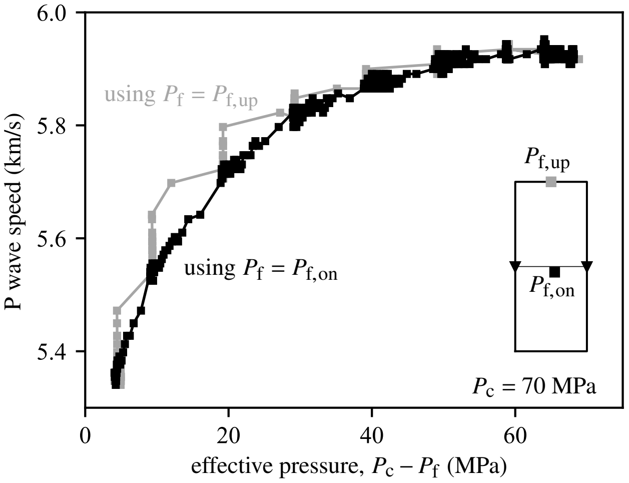


Figure S7: Evolution of the horizontal P wave velocity across the middle of the sample (see path indicated in the inset schematic) as a function of the Terzaghi effective pressure as measured at the upstream end of the sample (using $P_{\mathrm{f,up}}$, grey points) or at an intermediate position (using $P_{\mathrm{f,on}}$, black points), during a hydrostatic pressurisation at $P_{\mathrm{c}} = 70$ MPa and step-wise variations in $P_{\mathrm{f,up}}$.

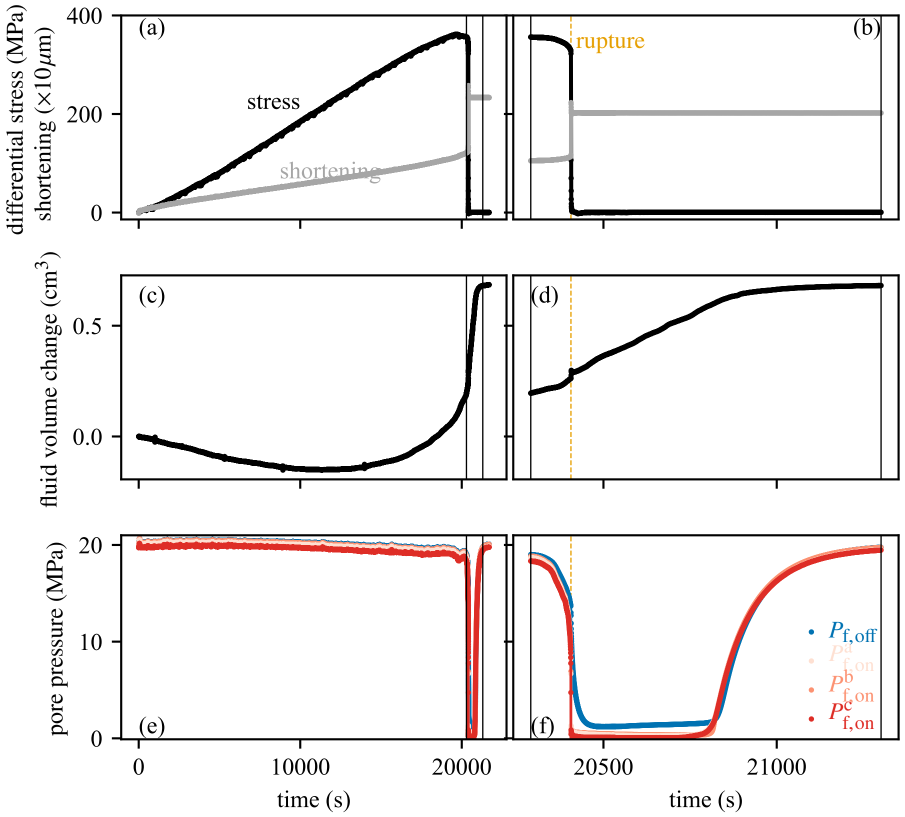


Figure S8: Test conducted at $P_c = 60$ MPa and $P_f = 20$ MPa. Differential stress and axial shortening (a,b), pore volume change (c,d) and on- and off-fault pore pressure (e,f) as a function of time during the triaxial rupture experiment. Panels (b,d,f) correspond to the time period marked between the thin vertical lines in panels (a,c,e). Pore pressure transducers are labelled as in Figure S1c.

# Results from the test conducted at $P_c = 60$ MPa and $P_f = 20$ MPa

# References

Carslaw, H. S. and J. C. Jaeger (1959), *Conduction of heat in solids*, 2nd edition, Oxford University Press, New York.

Passelègue, F. X., N. Brantut, and T. M. Mitchell (2018), Fault reactivation by fluid injection: Controls from stress state and injection rate, *Geophys. Res. Lett.*, 45, doi:10.1029/2018GL080470, 12837–12846.
